# Supplementary material for: Ab initio description of the Bi$_2$Sr$_2$CaCu$_2$O$_{8+\delta}$ electronic structure
Source: arXiv:2003.04034 ancillary file (2020-07-05)
Supplement: Supplementary file 1 [file bscco_supplemental.pdf]

# Supplemental material: *Ab initio* description of the $Bi_2Sr_2CaCu_2O_{8+\delta}$ electronic structure

Johannes Nokelainen[1,*], Christopher Lane[2,3], Robert S. Markiewicz[4], Bernardo Barbiellini[1,4], Aki Pulkkinen[5,1], Bahadur Singh[4], Jianwei Sun[6], Katariina Pussi[1], and Arun Bansil[4]

[1] *Department of Physics, School of Engineering Science, LUT University, FI-53850 Lappeenranta, Finland*
[2] *Theoretical Division, Los Alamos National Laboratory, Los Alamos, New Mexico 87545, USA*
[3] *Center for Integrated Nanotechnologies, Los Alamos National Laboratory, Los Alamos, New Mexico 87545, USA*
[4] *Physics Department, Northeastern University, Boston, Massachusetts 02115, USA*
[5] *Département de Physique and Fribourg Center for Nanomaterials, Université de Fribourg, CH-1700 Fribourg, Switzerland*
[6] *Department of Physics and Engineering Physics, Tulane University, Louisiana 70118 New Orleans, USA*
*johannes.nokelainen@lut.fi
†laneca@lanl.gov

## 1 $Bi_2Sr_2CuO_6$ (Bi2201)

We have also performed calculations on the $CuO_2$ monolayer compound Bi2201 which does not contain any calsium layers. Relaxing the structure gives a unit cell of 5.294 Å × 5.407 Å × 24.860 Å. The corresponding experimental values are 5.376(1) Å × 5.383(1) Å × 24.384(7) Å [97]. The agreement is reasonable, but not as good as in the case of Bi2212. Notably, the relaxed structure exhibits significant elongation in the *ab* plane. This feature of Bi2201 might be due to the doubling of the Bi/Cu ratio compared to Bi2212, so that the BiO zigzag chains include a greater reduction of the *a* axis (see the discussion in Sec. II A of the main text). In a physical sample this effect might be smaller due to the presence of type-B oxygen dopants, which would relieve the stress in the BiO layers. Also Bi atoms being substituted by other elements could result into this stress relief effect, as for example in Ref. [94] 20 % of the Bi atoms have been substituted with Ca.

The electronic structure of undoped Bi2201 is shown in Fig. 1 and compared with that of Bi2212. Three important differences between Bi2201 and Bi2212 can be observed as follows. (1) The self-doping is significantly stronger in Bi2201 because the bismuth pockets in Bi2201 reach further below $E_F$ (compared to Bi2212) and the Cu $d_{x^2-y^2}$ bands extend further above $E_F$. Also the energy gap in Cu $d_{x^2-y^2}$ is decreased with about 0.1 eV. Consequently, the Cu magnetic moment is only 0.395 $\mu_B$, which is 0.030 $\mu_B$ less than in Bi2212. These differences are due to the smaller number

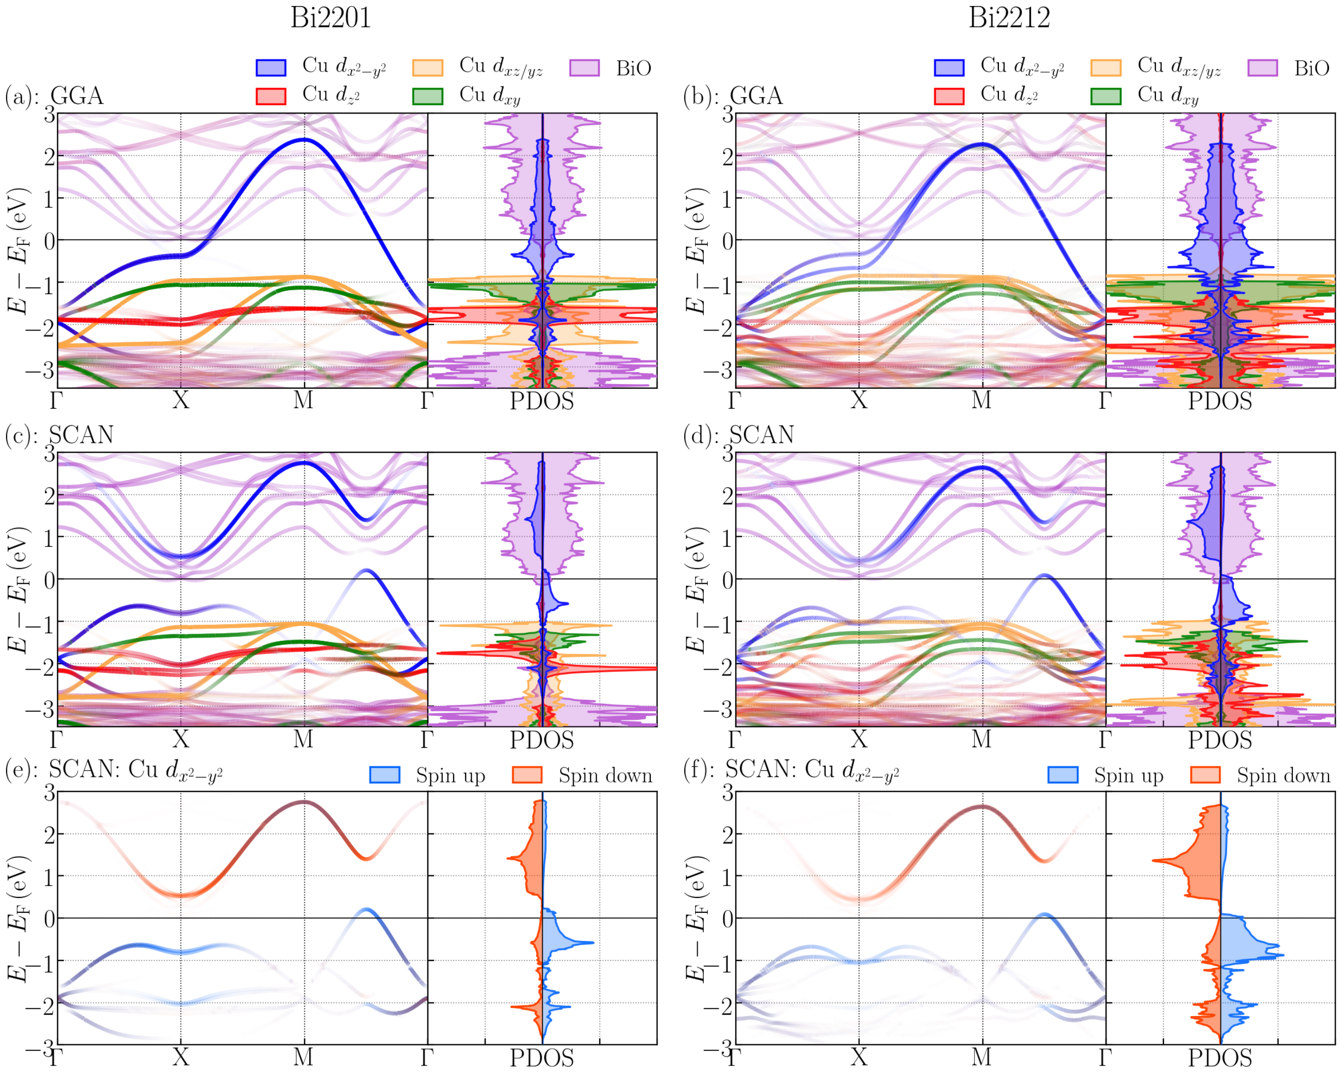


Figure 1: Electronic structure of Bi2201 (left) and Bi2212 (right). Panels (a) and (b) give the GGA band structure and the related DOS projected onto Cu orbitals and BiO layers. Panels (c) and (d) give the corresponding results based on SCAN data. The projections for Cu refer only to those sites that carry a positive magnetic moment (spin polarization is not shown in the band structure plots for simplicity). Panels (e) and (f) give the SCAN-based band structure and DOS of the magnetic $d_{x^2-y^2}$ orbitals. The band structures have been unfolded from the AFM $\sqrt{2} \times \sqrt{2}$ supercell to the primitive cell. The symmetry points $X$ and $M$ are given with respect to the Brillouin zone of the primitive cell.

of $CuO_2$ planes in Bi2201, so that the effective Bi/Cu ratio in Bi2201 is twice as large, which makes the self-doping due to Bi more prominent. (2) There is no bilayer splitting in Bi2201. As a result, there is only one van Hove singularity at $-0.6\,\mathrm{eV}$ instead of two singularities in Bi2212 at around $-0.65\,\mathrm{eV}$ and $-0.88\,\mathrm{eV}$. Moreover, the $d_{z^2}$ and $t_{2g}$ related peaks in the DOS are significantly sharper in Bi2201 compared to Bi2212. (3) Curiously, our estimation for the value of $U$ is $4.3\,\mathrm{eV}$, which is $0.4\,\mathrm{eV}$ less than in Bi2212. However, the value of Hund's splitting ($-1.34\,\mathrm{eV}$) in Bi2201 is almost equal to that of Bi2212.
